# Supplementary material for: Active mechanics reveal molecular-scale force kinetics in living oocytes
Source: arXiv:1510.08299 ancillary file (2018-02-08)
Supplement: Supplementary file 1 [file SM.pdf]

# Supplementary Material for "Active mechanics reveal molecular-scale force kinetics in living oocytes "

November 8, 2016

**Wylie W. Ahmed**[1,2,7], **Etienne Fodor**[3,7], **Maria Almonacid**[4,7], **Matthias Bussonnier**[2], **Marie-Helene Verlhac**[4], **Nir Gov**[5], **Paolo Visco**[3], **Frederic van Wijland**[3], **Timo Betz**[2,6]
1 Department of Physics, California State University, Fullerton, California 92831, USA
2 Laboratoire Physico Chimie Curie, Institut Curie, PSL Research University, CNRS UMR168, 75005, Paris, France; Sorbonne Universités, UPMC Univ Paris 06, 75005, Paris, France
3 Laboratoire Matiere et Systemes Complexes, UMR 7057, Universite Paris Diderot, 75013 Paris, France
4 CIRB, College de France, and CNRS-UMR7241 and INSERM-U1050, Equipe Labellisee Ligue Contre le Cancer, Paris F-75005, France
5 Department of Chemical Physics, Weizmann Institute of Science, 76100 Rehovot, Israel
6 Institute of Cell Biology, Center for Molecular Biology of Inflammation, Cells-in-Motion Cluster of Excellence, Münster University, Von-Esmarch-Strasse 56, D-48149 Münster, Germany
7 equally contributing authors
November 8, 2016

## 1 Simulations

To simulate the dynamics of the vesicles, we first approximate the power law memory kernel $\gamma(t) \propto t^{-\alpha}$ as a finite sum of exponential functions (Prony series): $\gamma(t) = \sum_i c_i \mathrm{e}^{-t/\sigma_i}/\sigma_i$. Following the methods developed in [2], it is possible, with $N$ exponential terms, to accurately approximate a power law decay over $N$ decades. Parameters $c_i$ and $\sigma_i$ are then given by,

$$\sigma_i = \frac{10^i}{\alpha}, \quad c_i = \frac{\kappa\zeta_\alpha^\alpha}{\Gamma(1-\alpha)} \frac{10^{-i(\alpha-1)}}{\alpha \sum_j 10^{-j\alpha} \mathrm{e}^{-\alpha/10^j}} \tag{1}$$

We approximate the power law kernel in the time window $\left[10^{N_-}, 10^{N_+ - 1}\right]$, where $N_- < 0 < N_+$, and $N = N_+ - N_- + 1$. Then, the index in the Prony series goes from $i = N_-$ to $i = N_+$.

With $\gamma$ a sum of $N$ exponential functions, it is possible to turn equations equations (1) and (2) from the main text into a $(2N+2)$-dimensional Markovian process for the variables $\left\{x, x_0, y_{N_-}, \dots, y_{N_+}, z_{N_-}, \dots, z_{N_+}\right\}$:

$$\sum_{i=N_-}^{N_+} \frac{c_i}{\sigma_i}(x - y_i) = -\kappa(x - x_0), \qquad \sum_{i=N_-}^{N_+} \frac{c_i}{\sigma_i}(x_0 - z_i) = \kappa\zeta_\alpha v_A, \tag{2}$$

$$c_i \frac{\mathrm{d}y_i}{\mathrm{d}t} = -\frac{c_i}{\sigma_i}(y_i - x) + \xi_i, \qquad \frac{\mathrm{d}z_i}{\mathrm{d}t} = -\frac{z_i - x_0}{\sigma_i}, \tag{3}$$

where the $\{\xi_i\}_i$ are the zero mean Gaussian noises with correlations $\langle \xi_i(t)\xi_j(t')\rangle = 2k_BTc_i\delta_{ij}\delta(t-t')$. By using Euler's methods to simulate this set of equations, the iterative equations take the following form in terms of the sampling time $\Delta t$,

$$y_i(t+\Delta t) = y_i(t) - \frac{\Delta t}{\sigma_i}\left(y_i(t) - x(t)\right) + \sqrt{\frac{2k_BT\Delta t}{c_i}}\eta, \quad z_i(t+\Delta t) = z_i(t) - \frac{\Delta t}{\sigma_i}\left(z_i(t) - x_0(t)\right) \tag{4}$$

$$x_0(t+\Delta t) = \frac{\kappa\zeta_\alpha v_A(t+\Delta t) + \sum_i c_i z_i(t+\Delta t)/\sigma_i}{\sum_i c_i/\sigma_i}, \quad x(t+\Delta t) = \frac{\kappa x_0(t+\Delta t) + \sum_i c_i y_i(t+\Delta t)/\sigma_i}{\kappa + \sum_i c_i/\sigma_i} \tag{5}$$

where $\eta$ is random Gaussian variable with zero mean and variance equal to 1, and $v_A$ is the stochastic process described earlier, which is computed according to the following rules:

$$v_A(t+\Delta t) = \begin{cases} v_A(t) & \text{if } v_A(t) \neq 0 \text{ with Pr. } 1-\Delta t/\tau \\ v_A(t) & \text{if } v_A(t) = 0 \text{ with Pr. } 1-\Delta t/\tau_0 \\ 0 & \text{if } v_A(t) \neq 0 \text{ with Pr. } \Delta t/\tau \\ U_{[-v,v]} & \text{if } v_A(t) = 0 \text{ with Pr. } \Delta t/\tau_0 \end{cases} \tag{6}$$

where $U_{[-v,v]}$ is a uniform random number between $-v$ and $v$ and $\tau_0 = \tau(1-p_{\text{on}})/p_{\text{on}}$ is the timescale over which the active burst is 0.

In order to mimic the experimental condition, we chose a sampling time $\Delta t = 10^{-4}$ s, and we aimed to simulate our process up to 10 s. Then, we have set $\{N_-, N_+\} = \{4, -2\}$, so that the power law memory kernel is well approximated in the time window$[10^{-4}, 10]$ s, with parameter values $\{\alpha, \kappa\zeta_\alpha^\alpha, N_-, N_+\} = \{0.6, 1, -4, 2\}$

Other parameters in the simulation were chosen according to the numerical fits over experimental data, and as listed in Table 1 where $p_{\text{on}} = 4\%$ and $v = 60\mu\text{m}\cdot\text{s}^{-1}$ where $p_{\text{on}} = \tau/(\tau+\tau_0)$ where $(\tau+\tau_0)$ is the total myosin-V step duration [3, 7] and $v$ is the amplitude of the active burst velocity calculated from $v = F/(\kappa\tau)$. We also took $k_BT = 4\times10^{-21}$ J.

We started the simulation with all variables set to 0 and waited for thermalization by running the simulation for $10^3$ time steps. We then start collecting position data $x$ in order to build the histogram for the probability distribution function of the position. A total of approximately $10^5$ samples were collected to arrive at the histogram in Figure 4 of the main text.

# Crossover to thermally dominated forces

The relative balance between intracellular mechanical properties and active forces determines the frequency at which nonequilibrium activity becomes evident ($S_{\text{cell}} > S_{\text{therm}}$). To illustrate this we explore how mechanical properties change the force spectrum (equation 6 and 7 of the main text). The total force spectrum is the sum of contributions from active forces and thermal forces, ($S_{\text{cell}} = S_{\text{active}} + S_{\text{therm}}$). Figure S4A shows the theoretical curves for the force spectrum measured in the present study. Here, we can observe that the magnitude of thermal and active forces is equal at 20 Hz (denoted by the purple diamond) and that thermal forces dominate the spectrum ($S_{\text{cell}} \approx S_{\text{therm}}$) at approximately 300 Hz (gray star). This also highlights that the active forces still contribute to the total force spectrum even when they are much smaller than the thermal forces. Now if the system is made softer by decreasing the coefficient of the viscoelastic memory kernel, $\gamma_\alpha = 0.2\cdot\gamma_\alpha(\text{WT})$, we see that thermal forces do not dominate until 1000 Hz (Figure S4B). Alternatively, if the system is made stiffer ($\gamma_\alpha = 5\cdot\gamma_\alpha(\text{WT})$)(Figure S4C), then thermal forces begin to dominate at much lower frequency (25 Hz, gray star). Therefore, by only changing the mechanical properties of the system by a small amount, the frequency at which thermal forces dominate can be changed dramatically.

# Laser tracking interferometry of endogenous vesicles

Laser tracking interferometry allows the displacement fluctuations of a rigid particle to be measured with high spatiotemporal resolution [4]. This technique assumes that the particle of interest is rigid. However, small endogenous particles in living cells may undergo shape fluctuations due to deformation or rotation that could affect the laser tracking signal. Therefore, we investigated the validity of using endogenous vesicles as probes for laser tracking interferometry and conclude that measured fluctuations are dominated by active displacements of the vesicle (details follow below).

We estimated the expected amplitude of vesicle deformation [1],

$$R\cdot\langle|u|\rangle = R\left[\frac{k_BT}{(\kappa(l+2)(l-1)l(l+1)+\sigma R^2(l+2)(l-1))}\right]^{1/2} \tag{7}$$

where $u$ is the deformation amplitude, $k_B T$ is thermal energy, $\kappa = 50 k_B T$ is the membrane bending stiffness, $\sigma = 5 \times 10^{-5}$ N/m is the membrane tension, $R = 500$ nm is the vesicle radius, and $l = 2$ is the dominant mode of deformation. The calculated vesicle deformation ($\sim 4$ nm) is an order of magnitude smaller than the measured fluctuations ($\sim 100$ nm) and thus we expect that our laser-tracking of vesicles is dominated by displacements.

To test this experimentally we used several approaches. First, we confirm that the signal:noise ratio for laser interferometry (as indicated by the slope of the QPD measurement) is similar for endogenous vesicles, a colloidal bead in a cultured cell, and a colloidal bead in an index matched solution (Figure S5). Second, we perform active microrheology on a vesicle in a living oocyte at different laser powers. If vesicle deformation were significant, then the measured complex shear modulus would exhibit a systematic difference depending on laser power. Our measurements show that the moduli do not depend on laser power (Figure S6). Third, we deplete ATP in oocytes by treatment with 2mM sodium azide + 10 mM deoxyglucose to remove motion generated by active biological processes. If the signal contribution from passive vesicle deformations is comparable to displacements then we expect the amplitude of the measured fluctuations in ATP depleted cells to be comparable to the WT condition. Our measurements show that measured fluctuations in the ATP depleted case are an order of magnitude (or more) lower than in WT oocytes for all frequencies measured (Figure S7). Third, we isolated vesicles from oocytes by crushing them between two glass coverslips resulting in ruptured cells and expulsion of cytoplasmic contents into the surrounding medium. Isolated vesicles were immobilized due to adhesion to the poly-l-lysine coated coverslip. If vesicle deformation significantly influenced our laser interferometry measurement, then we expect the measured fluctuations of an immobilized isolated vesicle to be larger than an immobilized (rigid) colloidal bead. Our measurements show that measured fluctuations of an immobilized vesicle are comparable to an immobilized bead (Figure S8) (high-frequency deviation results from shot noise due to a lower refractive index of the vesicle relative to the bead). Fourth, we measured the response of immobilized vesicles by applying force with high laser power (120 mW). This quantifies the response due to only vesicle deformation (since it is immobilized). Our measurements show that deformation of an immobilized isolated vesicle (red data points) is more than an order of magnitude smaller than the response measured with vesicles in WT oocytes (blue data points) (Figure S9). Therefore, in living cells, our measurements are dominated by vesicle displacements and not deformations. Lastly, we created synthetic vesicles via electroformation as done previously [1] to allow direct measurement in a well-controlled environment. Vesicles were placed in a hypertonic environment (175 mOsm/kg sucrose inner buffer and 185 mOsm/kg NaCl outer buffer) to promote membrane fluctuations. The power spectral density of synthetic vesicles ($\sim$1 $\mu$m) is fit well by the theory for rigid beads (Figure S10 (left)) but is not fit well by the theory for deformable vesicles as seen at intermediate frequencies (Figure S10 (right)). Note that the extracted fitting parameters for the rigid bead theory agree with expected values, but to obtain a fit for the vesicle theory the fitting parameters must take on unrealistic values for our experimental conditions. Together, these experiments suggest that small vesicles behave indistinguishably from rigid particles in our experiments and serve as suitable probes for laser tracking interferometry.

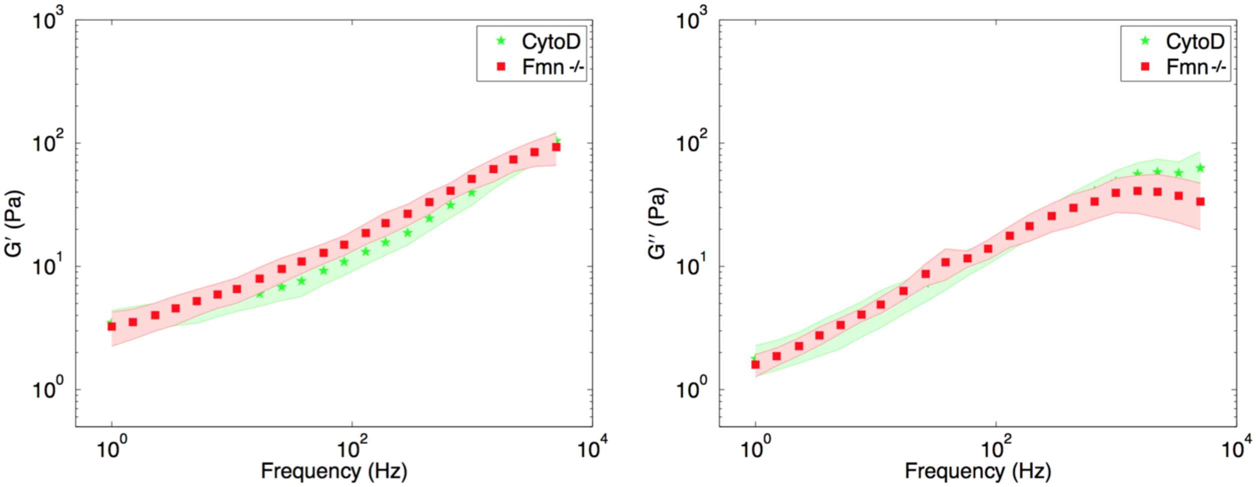


Figure S1: Viscoelastic shear moduli of Fmn -/- oocytes are not significantly different from WT + Cytochalasin-D oocytes. To confirm that actin filaments do not provide significant mechanical resistance, we treated WT oocytes with cytochalasin-D (1 $\mu$g/ml) for 2 hours. Subsequent AMR measurements showed their mechanical properties were not different than Fmn -/- oocytes. ($n_{\mathrm{Fmn}-/-} = 23$ and $n_{\mathrm{cytoD}} = 16$; shaded region indicates standard error of the mean)

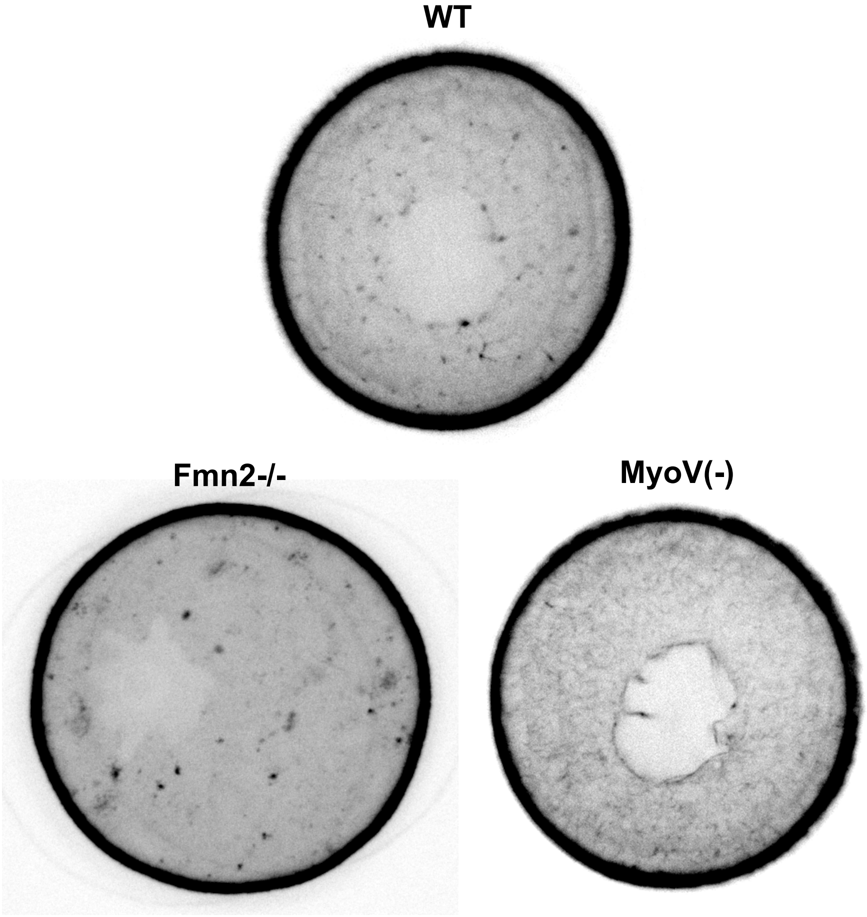


Figure S2: The actin meshwork was visualized with GFP-UtrCH to show the actin meshwork. WT oocytes exhibit a network of actin positive vesicles connected by actin filaments to create a meshwork. Fmn2 -/- exhibited punctate actin but no visible meshwork. MyoV(-) exhibit an increased density actin meshwork relative to WT. Images were captured at 37 degrees Celsius using a 40x objective (1.25NA) on a Leica DMI6000B microscope enclosed in a thermostatic chamber (Life Imaging Service) equipped with a CoolSnap HQ2/CCD-camera (Princeton Instruments) coupled to a Sutter filter wheel (Roper Scientific) and a Yokogawa CSU-X1-M1 spinning disc. (oocyte diameter is 80 $\mu$m)

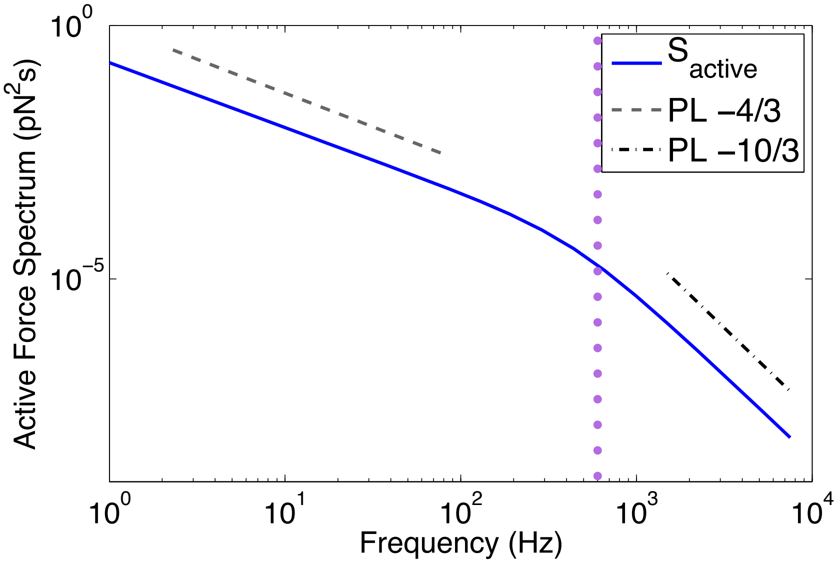


Figure S3: The active force spectrum shows two distinct power-law (PL) behaviors at low ($f^{-2\alpha}$) and high frequency ($f^{-2\alpha-2}$) compatible with the experimentally measured $\alpha \sim 2/3$.

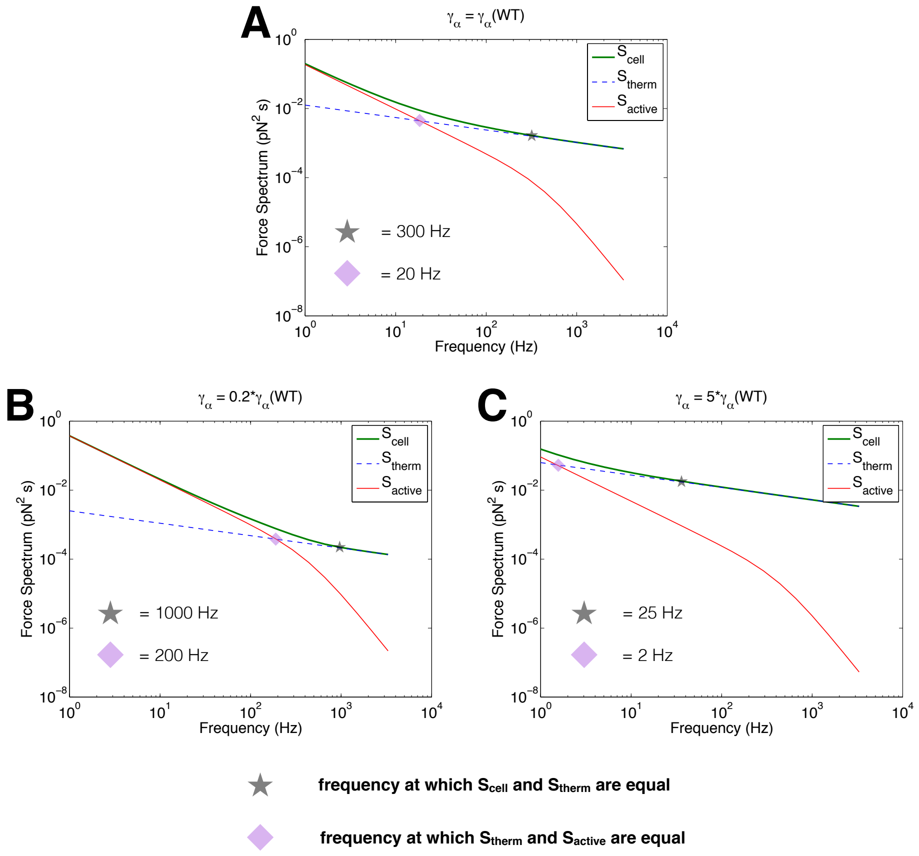


Figure S4: Force spectrum depends on the mechanical properties of the system. (A) The theoretical curves for the force spectrum measured in the experiments in this study where the coefficient of the memory kernel is $\gamma_\alpha = \gamma_\alpha(\mathrm{WT})$ and the thermal forces dominate at around 300 Hz. (B) The mechanical properties are softened by $\gamma_\alpha = 0.2 \cdot \gamma_\alpha(\mathrm{WT})$ and the frequency where thermal forces dominate is shifted up to 1000 Hz. (C) The mechanical properties are stiffened by $\gamma_\alpha = 5 \cdot \gamma_\alpha(\mathrm{WT})$ and the thermal forces dominate at 25 Hz.

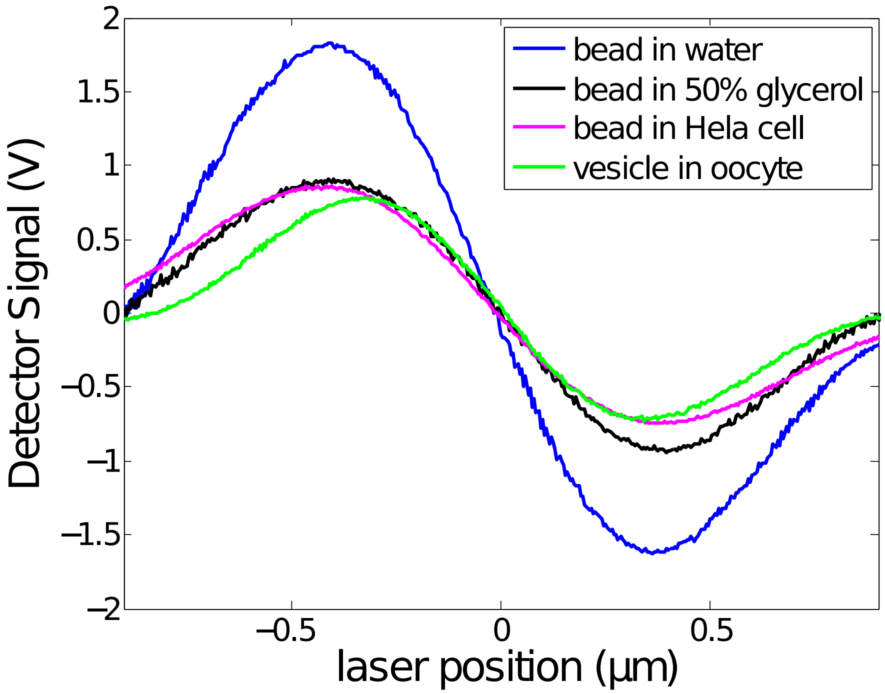


Figure S5: QPD voltage vs. laser position for various conditions. The slope of the central linear region is indistinguishable between a vesicle (diameter of approximately 1 micron) in an oocyte (green), a 1 micron colloidal bead in a Hela cell (magenta), and a 1 micron colloidal bead in an index matched solution of 50:50 water:glycerol. For comparison, the slope of a 1 micron colloidal bead in pure water is significantly steeper due to the higher difference in index of refraction. This measurement shows that the signal:noise ratio for the QPD measurements is similar for endogenous vesicles and colloidal beads in cells and index matched media.

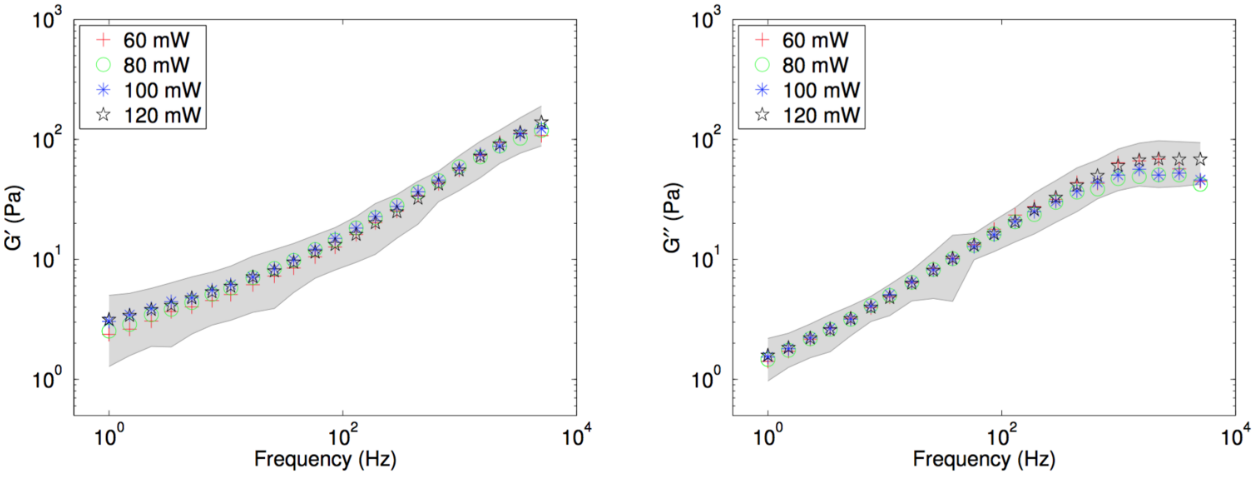


(a) elastic moduli

(b) viscous moduli

Figure S6: Viscoelastic shear moduli of oocytes is not affected by the laser power used for active microrheology. Measurements were performed on the same vesicle at different laser powers and a representative example is shown. ($n = 23$; shaded region indicates standard deviation of all measurements)

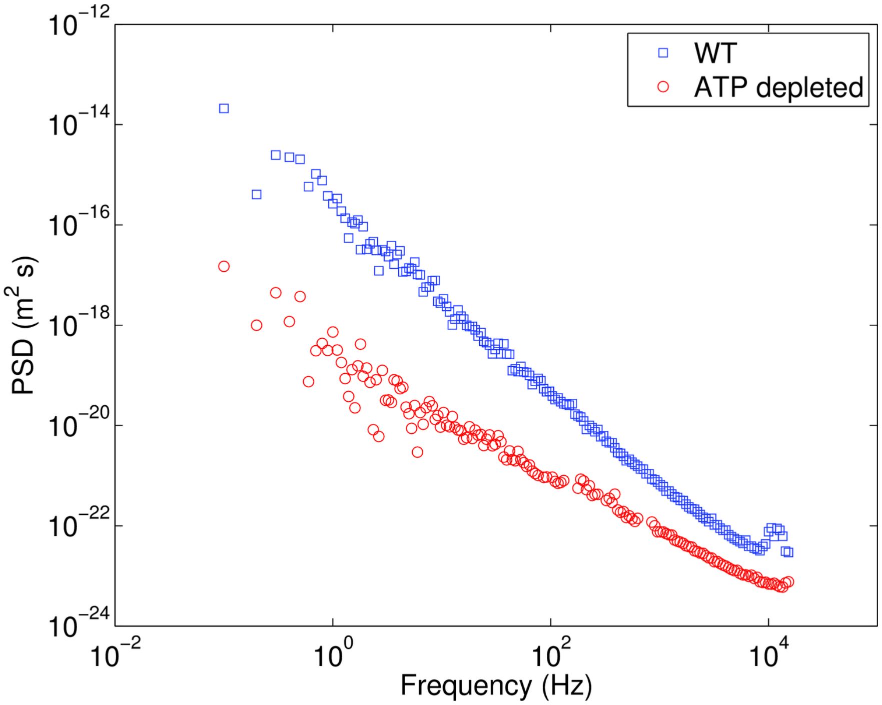


Figure S7: Power spectral density of measured fluctuations in ATP depleted oocytes are significantly lower than in WT oocytes. (local peaks from resonant frequencies of piezo stage feedback have been removed from data)

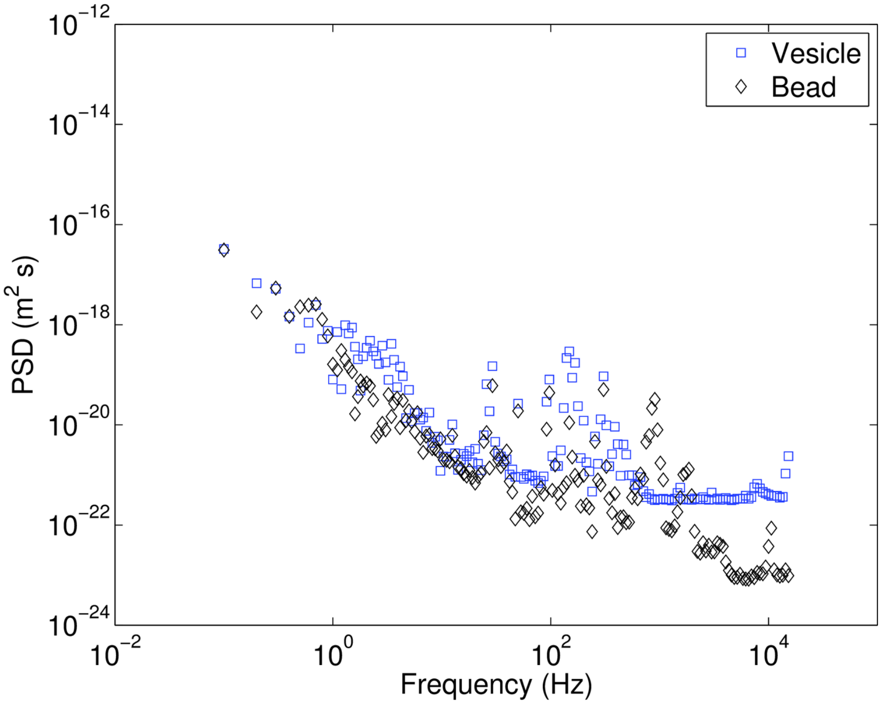


Figure S8: Power spectral density of measured fluctuations in an isolated oocyte vesicle are not significantly different than a colloidal bead (both of ∼1 micron diameter).

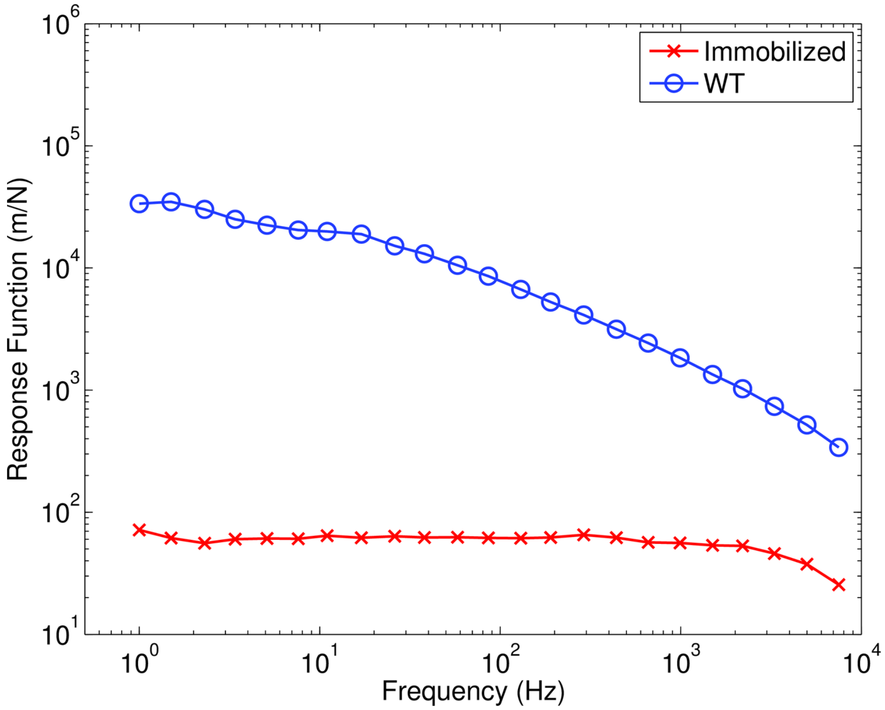


Figure S9: The force response of an isolated and immobilized vesicle is at least an order of magnitude smaller than for freely moving vesicles in WT oocytes. The forced response was measured on a $\sim 1$ micron diameter vesicle at 120 mW laser power. This measurement suggests that deformations of the vesicle itself are a small contribution to our measured signal. ($n_{immobilized} = 8$, $n_{WT} = 8$)

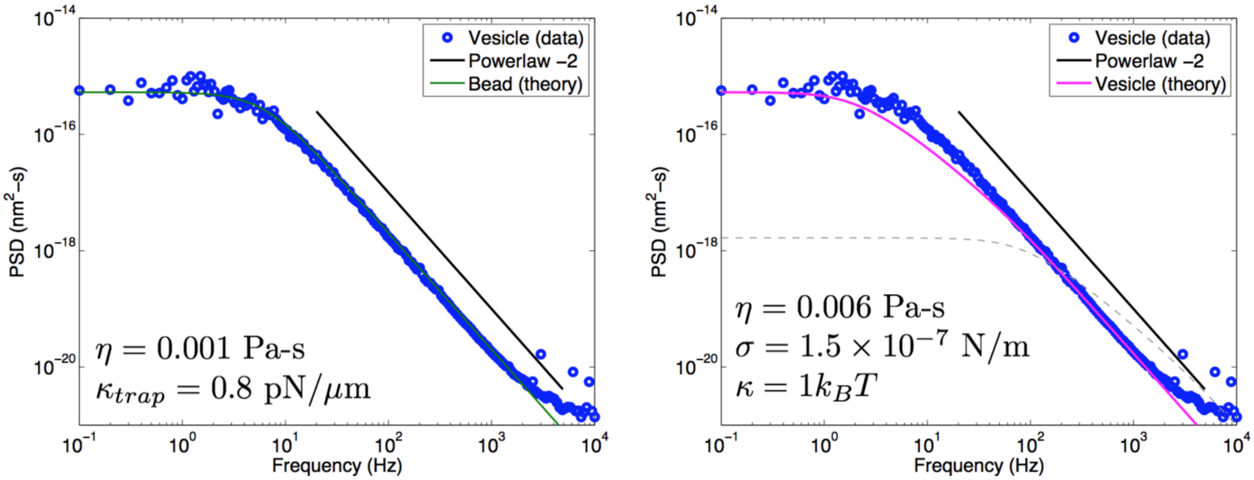


Figure S10: The power spectral density (PSD) of a trapped synthetic vesicle ($\sim$ 1 micron at 5 mW laser power) made by electroformation [1] is compared with the theory for a rigid bead (left) and a deformable vesicle (right). (Left) The measured data for a vesicle is fit well by the theory for a rigid bead trapped in a harmonic potential [5] and the extracted fit parameters ($\eta = 0.001$ Pa-s, $\kappa_{trap} = 0.8$ pN/$\mu$m) agree with the viscosity of water and the optical trap stiffness. (Right) The measured data is not fit well by the theory for a deformable vesicle [6], showing deviation at intermediate frequencies and unrealistic fit parameters. Note that for the vesicle theory the extracted viscosity ($\eta = 0.006$ Pa-s) is six times higher than expected for water and the membrane tension ($\sigma = 1.5 \times 10^{-7}$ N/m) and membrane bending stiffness ($\kappa = 1k_BT$) are an order of magnitude lower than expected for these vesicles [1]. The PSD expected for a vesicle with realistic physical parameters ($\eta = 0.001$ Pa-s, $\sigma = 1 \times 10^{-6}$ N/m, and $\kappa = 10k_BT$) is shown as a dotted-gray line [1]. This measurement suggests that small vesicles are best approximated by the rigid bead theory (left) and are suitable for laser-tracking interferometry. ($n = 16$)

# References


[1] Timo Betz and Cécile Sykes. Time resolved membrane fluctuation spectroscopy. *Soft Matter*, 8(19):5317–5326, 2012.

[2] Thierry Bochud and Damien Challet. Optimal approximations of power laws with exponentials: application to volatility models with long memory. *Quantitative Finance*, 7(6):585–589, dec 2007.

[3] G Cappello, P Pierobon, C Symonds, L Busoni, JC Gebhardt, M Rief, and J Prost. Myosin V stepping mechanism. *Proc Natl Acad Sci U S A*, 104:15328–33, Sep 2007.

[4] F Gittes and CF Schmidt. Interference model for back-focal-plane displacement detection in optical tweezers. *Opt Lett*, 23:7–9, Jan 1998.

[5] Frederick Gittes and C. F. Schmidt. Thermal noise limitations on micromechanical experiments. *European Biophysics Journal*, 27(1):75–81, jan 1998.

[6] Scott T. Milner and S. A. Safran. Dynamical fluctuations of droplet microemulsions and vesicles. *Phys. Rev. A*, 36(9):4371–4379, nov 1987.

[7] Sotaro Uemura, Hideo Higuchi, Adrian O Olivares, Enrique M De La Cruz, and Shin'ichi Ishiwata. Mechanochemical coupling of two substeps in a single myosin V motor. *Nat Struct Mol Biol*, 11(9):877–883, aug 2004.
